# Supplementary material for: Multiplicative local linear hazard estimation and best one-sided cross-validation
Source: arXiv:1710.05575 ancillary file (2017-10-16)
Supplement: Supplementary file 1 [file SuppPub1.pdf]

# Supplementary material for:
## Multiplicative local linear hazard estimation and best one-sided cross-validation

# 1 Details of asymptotics and proofs

## 1.1 Assumptions

A1. *The kernels $K$ and $L$ are compactly supported (i.e. the support is contained in $[-C_K, C_K]$ for some constants $C_K > 0$). The kernels are continuous on $I\!R \backslash \{0\}$ and have one-sided derivatives that are Hölder continuous on $I\!R^- = \{x : x < 0\}$ and $I\!R^+ = \{x : x > 0\}$, that is there exist constants $c$ and $d$ such that $|\phi(x) - \phi(y)| \le c|x-y|^d$ for $x, y < 0$ or $x, y > 0$ with $\phi$ equal to $K'$ or $L'$. The left and right-sided derivatives differ at most on a finite set. The kernel $K$ is symmetric.*

*A2. For the expected exposure function $\gamma(t) = n^{-1}E[Y(t)]$ it holds that $\gamma \in C_2([0,T])$, that it is strictly positive for $t \in [0,T]$, and that*

$$\begin{aligned} \sup_{s\in[0,T]} |Y(s)/n - \gamma(s)| &= o_P\left((\log n)^{-1}\right), \\ \sup_{s,t\in[0,T],|t-s|\le C_K b} |[Y(t) - Y(s)]/n - [\gamma(t) - \gamma(s)]| &= o_P\left((nb\log n)^{-1/2}\right), \end{aligned}$$

*where the constant $C_K$ is defined in assumption A1.*

*A2'. For the expected exposure function $\gamma(t) = n^{-1}E[Y(t)]$ it holds that $\gamma \in C_2([0,T])$, that it is strictly positive for $t \in [0,T]$, and that*

$$\begin{aligned} \sup_{s\in[0,T]} |Y(s)/n - \gamma(s)| &= o_P((\log n)^{-1}), \\ \sup_{s,t\in[0,T],|t-s|\le C_K b} |[Y(t) - Y(s)]/n - [\gamma(t) - \gamma(s)]| &= o_P((nb)^{-1}), \end{aligned}$$

*where the constant $C_K$ is defined in assumption A1.*

*A3. It holds that $\alpha \in C_2([0,T])$, $w \in C_1([0,T])$. The second derivative of $\alpha$ is Hölder continuous with exponent $d > 0$.*

*A3'. It holds that $\alpha \in C_4([0,T])$, $w \in C_1([0,T])$. The fourth derivative of $\alpha$ is Hölder continuous with exponent $d > 0$.*

## 1.2 Central limit theorem for martingales

Proposition 4.2.1. in Ramlau-Hansen (1983) establishes a central limit theorem for martingales. We recall here the version of the theorem that is given in Hiabu et al. (2016), that is:

**Theorem 3** *Consider a predictable process $Z_n(t)$ and assume that for some $\sigma^2 \geq 0$*

$$\int Z_n^2 Y(t)\alpha(t)dt = \sigma^2 + o_P(1), \qquad \int Z_n^2 I\left\{Z_n^2 > \epsilon\right\} Y(t)\alpha(t)dt = o_P(1), \quad \epsilon > 0.$$

*Then, it holds that $\int Z_n(u)dM(u) \to N\left(0,\sigma^2\right)$, in distribution, as $n \to \infty$.*

## 1.3 Asymptotics of bandwidth selectors for a local linear estimator

Let consider the local linear hazard estimator, $\widehat{\alpha}_{b,L}^{\mathrm{LL}}$, with bandwidth $b$ and a generic kernel $L$, given by

$$\widehat{\alpha}_{b,L}^{\mathrm{LL}}(t) = \sum_{i=1}^{n} \int_0^T \bar{L}_{t,b}(t-s)dN_i(s), \tag{1}$$

with stochastic local linear kernel

$$\bar{L}_{t,b}(t-s) = \frac{a_{2,L}(t) - a_{1,L}(t)(t-s)}{a_{0,L}(t)a_{2,L}(t) - (a_{1,L}(t))^2} L_b\left(t-s\right), \tag{2}$$

where $L_b(u) = b^{-1}L(u/b)$ and $a_{j,L}(t) = \int_0^T L_b\left(t-s\right)(t-s)^j Y(s)ds$, for $j = 0, 1, 2$.

Recall the decomposition:

$$\widehat{\alpha}_{b,L}^{\mathrm{LL}}(t) - \alpha(t) = V_{b,L}^{\mathrm{LL}}(t) + B_{b,L}^{\mathrm{LL}}(t), \tag{3}$$

where

$$\begin{aligned} B_{b,L}^{\mathrm{LL}}(t) &= \int_0^T \bar{L}_{t,b}(t-s)\left(\alpha(s)-\alpha(t)\right)Y(s)ds, \\ V_{b,L}^{\mathrm{LL}}(t) &= \int_0^T \bar{L}_{t,b}(t-s)dM(s). \end{aligned} \tag{4}$$

To prove Theorem 1 we first state a uniform expansion for the ISE. The ISE of the local linear estimator in (1) is defined as

$$\Delta_L^{\mathrm{LL}}(b) = n^{-1}\int_0^T \left(\widehat{\alpha}_{b,L}^{\mathrm{LL}}(t)-\alpha(t)\right)^2 w(t)Y(t)dt.$$

Following Gámiz et al. (2016) we assume that $\widehat{b}_{\mathrm{ISE},L}^{\mathrm{LL}}$ is defined as the minimizer of $\Delta_L^{\mathrm{LL}}$ over the interval $I_n^{\mathrm{LL}} = \left[c_1 n^{-1/5}, c_2 n^{-1/5}\right]$, where constants $0 < c_1 < c_2$ are chosen such that $c_1 < C_{0,L}^{\mathrm{LL}} < c_2$, where is $C_{0,L}^{\mathrm{LL}}$ given by

$$C_{0,L}^{\mathrm{LL}} = \left[\frac{R\left(\bar{L}^*\right)\int \alpha(t)w(t)dt}{\mu_2^2\left(\bar{L}^*\right)\int \left(\alpha''(t)\right)^2\gamma(t)w(t)dt}\right]^{1/5}.$$

Here $\mu_j(L) = \int u^j L(u)du$, for $j = 1,2$, $R(L) = \int L^2(u)du$, and $\bar{L}^*$ is the equivalent kernel

$$\bar{L}^*(u) = \frac{\mu_2(L)-\mu_1(L)u}{\mu_2(L)-\mu_1(L)^2}L(u). \tag{5}$$

To simplify the notation hereafter in this section we remove the superscript LL and write $\widehat{\alpha}_{b,L}^{\mathrm{LL}} = \widehat{\alpha}_{b,L}$, $\Delta_L^{\mathrm{LL}} = \Delta_L$, $B_{b,L}^{\mathrm{LL}} = B_{b,L}$, $V_{b,L}^{\mathrm{LL}} = V_{b,L}$, $I_n^{\mathrm{LL}} = I_n$ and $C_{0,L}^{\mathrm{LL}} = C_{0,L}$.

### Asymptotic expansion of the ISE

**Lemma 4** *Under Assumptions A1–A3, we have the following expansion of the ISE of the local linear estimator with kernel $L$ and bandwidth $b$,*

$$\Delta_L(b) = M_L(b) + o_P((nb)^{-1}) = M_L(b) + o_P(n^{-4/5}),$$

*uniformly for $b \in I_n$, where*

$$M_L(b) = b^4\frac{\mu_2^2\left(\bar{L}^*\right)}{4}\int \left(\alpha''(t)\right)^2\gamma(t)w(t)dt + (nb)^{-1}R\left(\bar{L}^*\right)\int \alpha(t)w(t)dt.$$

*Proof.*

Using the decomposition of the error in (3), we can expand the ISE, $\Delta_L$, as

$$\begin{aligned}\Delta_L(b) &= n^{-1}\int_0^T \left(V_{b,L}(t)+B_{b,L}(t)\right)^2 w(t)Y(t)dt = \\ &= n^{-1}\int_0^T \left(V_{b,L}(t)\right)^2 w(t)Y(t)dt + 2n^{-1}\int_0^T V_{b,L}(t)B_{b,L}(t)w(t)Y(t)dt + \\ &+ n^{-1}\int_0^T \left(B_{b,L}(t)\right)^2 w(t)Y(t)dt.\end{aligned}$$

with $V_{b,L}(t)$ and $B_{b,L}(t)$ given in (4).

We cannot directly apply the specified above martingale central limit theorem (Theorem 3) to $\Delta_L$ because the corresponding integrands in the first two terms are not predictable, that is, values of $Y(s)$ for $s > t$ appear in the terms $a_{j,L}$ ($j = 0,1,2$) involved in the definition of $\bar{L}_{t,b}$. Following similar arguments as in Gámiz et al. (2016) we define

$$V^*_{b,L}(t) = \int_0^T \bar{L}^+_{t,b}(t-s)dM(s),$$

where $\bar{L}^+_{t,b}(t-s)$ is defined as in (2) but replacing $Y(s)$ by $Y(t) + n\left\{\gamma(s)-\gamma(t)\right\}$ in the corresponding integrands:

$$\bar{L}^+_{t,b}(t-s) = \frac{a^+_{2,L}(t) - a^+_{1,L}(t)(t-s)}{a^+_{0,L}(t)a^+_{2,L}(t) - \left(a^+_{1,L}(t)\right)^2} L_b(t-s), \tag{6}$$

with

$$a^+_{j,L}(t) = \int_0^T L_b(t-s)(t-s)^j\left[Y(t) + n\left\{\gamma(s)-\gamma(t)\right\}\right]ds,$$

Then we replace $\bar{L}_{t,b}$ by $\bar{L}^+_{t,b}$ in the expression of the variance. From Assumption A2 we have that $n^{-1}\left(a_{j,L}(t) - a^+_{j,L}(t)\right) = o_P\left\{(nb\log n)^{-1/2}\right\}$, then there exist a constant $C > 0$ such that $\sup_{s,t}\left|\bar{L}_{t,b}(s) - \bar{L}^+_{t,b}(s)\right| \leq Cn^{-1}(nb\log n)^{-1/2}b^{-1} = o_P\left\{(nb\log n)^{-1/2}\right\}$. This gives that

$$(nb\log n)^{1/2}\left|V^*_{b,L}(t)-V_{b,L}(t)\right| = o_P(1) \tag{7}$$

uniformly for $0\le t\le T$ and $b\in I_n$. The integrand in $V^*_{b,L}$ is predictable. Moreover we use Assumption A2, and (7), as well as $\sup\left|V^*_{b,L}(t)\right| = o_P\left\{(nb)^{-1/2}(\log n)^{1/2}\right\}$, and that $\sup|B_{b,L}(t)| = o_P\left\{(nb)^{-1/2}\right\}$, then we write

$$\begin{aligned}\Delta_L(b) &= \int_0^T \left(V^*_{b,L}(t)\right)^2 w(t)\gamma(t)dt + 2\int_0^T V^*_{b,L}(t)B_{b,L}(t)w(t)\gamma(t)dt + \\ &+ \int_0^T \left(B_{b,L}(t)\right)^2 w(t)\gamma(t)dt + o_P\left(n^{-4/5}\right)\end{aligned}$$

uniformly for $b\in I_n$. Focusing on the first term and changing the order of the integrals we can write

$$\int_0^T \left(V^*_{b,L}(t)\right)^2 w(t)\gamma(t)dt = \int_0^T\int_0^T \bar{H}^+_{L,b}(s,u)dM(s)dM(u) \tag{8}$$

with $\bar{H}^+_{L,b}(s,u)=\int_0^T \bar{L}^+_{t,b}(t-s)\bar{L}^+_{t,b}(t-u)w(t)\gamma(t)dt$; so can see (8) as a double integral of a predictable function with respect to martingale. We can subtract the diagonal term and decompose it as a sum, $\int_0^T\left(V^*_{b,L}(t)\right)^2 w(t)\gamma(t)dt = S_{L,1}(b)+T_{L,1}(b)$, where

$$\begin{aligned}S_{L,1}(b) &= \int_0^T\int_0^T \bar{H}^+_{L,b}(s,u)dM(s)dM(u) - \int_0^T \bar{H}^+_{L,b}(u,u)\alpha(u)Y(u)du,\\ T_{L,1}(b) &= \int_0^T \bar{H}^+_{L,b}(u,u)\alpha(u)Y(u)du.\end{aligned}$$

Moreover, for the second and third terms of $\Delta_L(b)$, we define

$$\begin{aligned}S_{L,2}(b) &= 2\int_0^T\left[\int_0^T \bar{L}^+_{t,b}(t-s)B_{b,L}(t)w(t)\gamma(t)dt\right]dM(s)\\ T_{L,2}(b) &= \int_0^T \left(B_{b,L}(t)\right)^2 w(t)\gamma(t)dt\end{aligned}$$

First we show that $S_{L,1}(b) = O_P\left(n^{-4/5}\right)$ and $S_{L,2}(b) = O_P\left(n^{-4/5}\right)$, uniformly for $b \in I_n$. To do it we define the martingale

$$S_{n,1,t}(x) = n^{4/5} \int_0^t \int_0^t \bar{H}^+_{L,xn^{-1/5}}(u,v)dM(u)dM(v) - n^{4/5} \int_0^t \bar{H}^+_{L,xn^{-1/5}}(u,u)\alpha(u)Y(u)du,$$

which can be expressed as

$$S_{n,1,t}(x) = n^{4/5} \int_0^t \int_0^v \left(\bar{H}^+_{L,xn^{-1/5}}(u,v) + \bar{H}^+_{L,xn^{-1/5}}(v,u)\right) I(u \neq v)dM(u)dM(v)$$

for $x \in [c_1, c_2]$; and the martingale

$$S_{n,2,t}(x) = n^{4/5} \int_0^t \delta_{L,xn^{-1/5}}(u)dM(u),$$

with $\delta_{L,xn^{-1/5}}(u) = 2\int_0^T \bar{L}^+_{xn^{-1/5},t}(t-u)B_{b,L}(t)w(t)\gamma(t)dt$.

To conclude that $S_{L,1}\left(xn^{-1/5}\right) = o_P\left(n^{-4/5}\right)$ we prove that $\sup_{x\in[c_1,c_2]} |S_{L,1,T}(x)| = o_P(1)$. To get this we can apply Theorem 3 for $\sigma^2 = 0$ and similar arguments as in Gamiz et al. (2016) to write $S_{n,1,t}(x) = \int_0^t Z_n(u,x)dM(u)$, where we denote $Z_n(u,x) = \int_0^u 2n^{4/5}\bar{H}^+_{L,xn^{-1/5}}(u,v)I(u \neq v)dM(v)$, and obtain pointwise convergence to zero.

A similar argument on $S_{2,n,t}$ provides $S_{L,2}\left(xn^{-1/5}\right) = o_P\left(n^{-4/5}\right)$. The uniform convergence to zero follows from the tightness of function $S_{n,1,T}(z)$ and $S_{n,2,T}(z)$ (Billingsley, 1968). Hence we conclude that

$$S_{L,1}(b) = o_P\left(n^{-4/5}\right), \text{ and } S_{L,2}(b) = o_P\left(n^{-4/5}\right),$$

uniformly in $b \in I_n$.

To finish the proof, using Assumptions A1–A3 we can get the following asymptotic approximations of $a^+_{j,L}(t)$, for $j = 0, 1, 2$, that is,

$$n^{-1}a^+_{j,L}(t) = \gamma(t)c_{j,L}(t) - \gamma'(t)c_{j+1,L}(t) + o_P\left(\log(n)^{-1}\right),$$

where we define $c_{j,L}(t) = \int_0^T L_b(t-s)(t-s)^j ds$. We can use this to show that the kernel $\bar{L}^+(t-s)$ is equivalent to $\dfrac{c_2(t) - c_1(t)(t-s)}{c_2(t)c_0(t) - c_1^2(t)} L_b(t-s)\{n\gamma(t)\}^{-1}$. Now it is not difficult to obtain that

$$T_{L,1}(b) = (nb)^{-1} R\left(\bar{L}^*\right) \int \alpha(t)w(t)dt + o_P\left((nb)^{-1}\right),$$

and

$$T_{L,2}(b) = b^4 \frac{\mu_2^2\left(\bar{L}^*\right)}{4} \int \left(\alpha''(t)\right)^2 \gamma(t)w(t)dt + o_P\left(b^4\right).$$

Putting all together, we get the asymptotic expression of the ISE $\Delta_L(b) = M_L(b) + o_P\left(n^{-4/5}\right)$, uniformly for $b \in I_n$. □

### Consistency of cross-validation and BO-validation

The following lemma proves consistency of the cross-validated bandwidth $\widehat{b}_{\mathrm{CV},L}$ for a general kernel $L$, and as a consequence the consistency of the BO-validated bandwidth.

**Lemma 5** *Under assumptions A1–A3, we have that* $\widehat{b}_{\mathrm{CV},L} = b_{\mathrm{MISE},L} + o_P\left(n^{-1/5}\right)$.

*Proof.* First we write the ISE in terms of the cross-validation score, $\widehat{Q}_L(b)$,

$$\widehat{Q}_L(b) = n^{-1}\left\{\sum_{i=1}^n \int_0^T \left[\widehat{\alpha}_{b,L}(s)\right]^2 Y_i(s)w(s)ds - 2\sum_{i=1}^n \int_0^T \widehat{\alpha}_{b,L}^{[i]}(s)w(s)dN_i(s)\right\}, \qquad (9)$$

as

$$\begin{aligned}\Delta_L(b) = \widehat{Q}_L(b) \;&+\; n^{-1}\int \alpha^2(s)Y(s)w(s)ds - 2n^{-1}\int \widehat{\alpha}_{b,L}(s)\alpha(s)Y(s)w(s)ds + \\ &+\; 2n^{-1}\int \widehat{\alpha}_{b,L}^{-}(s)w(s)dN(s).\end{aligned}$$

with $\widehat{\alpha}_{b,L}^{-}(s) = \int_0^T \bar{L}_{t,b}(t-s)I(s \neq t)dN(t)$. We can decompose the last term on the right hand side of the previous expression, and thus write

$$\Delta_L(b) = \widehat{\Delta}_L(b) + D_L(b)$$

where

$$\widehat{\Delta}_L(b) = \widehat{Q}_L(b) + n^{-1}\int \alpha^2(s)Y(s)w(s)ds + 2n^{-1}\int \alpha(s)dM(s).$$

and

$$\begin{aligned} D_L(b) &= 2n^{-1}\int \left(\widehat{\alpha}_{b,L}^{-}(s) - \widehat{\alpha}_{b,L}(s)\right)\alpha(s)Y(s)w(s)ds + 2n^{-1}\int \left(\widehat{\alpha}_{b,L}^{-}(s) - \alpha(s)\right)w(s)dM(s) \\ &= 2n^{-1}\int \left(\widehat{\alpha}_{b,L}^{-}(s) - \alpha(s)\right)w(s)dM(s). \end{aligned} \tag{10}$$

Note that $\widehat{\Delta}_L(b)$ has the same minimizer than $\widehat{Q}_L(b)$, then it is sufficient to show that $D_L(b) = o_P\left(n^{-4/5}\right)$, uniformly for $b \in I_n$, which can be obtained by similar arguments as Lemma 2 of Gamiz et al. (2016). Then we deduce that $\widehat{b}_{\mathrm{CV},L} = b_{\mathrm{MISE},L} + o_P\left(n^{-1/5}\right)$.

□

**Remark 1** *From Lemma 5 it follows the consistency of DO-validation since we have that* $\widehat{b}_{\mathrm{DO},K} = \frac{\varrho}{2}\left(\widehat{b}_{\mathrm{CV},K_{\mathrm{L}}} + \widehat{b}_{\mathrm{CV},K_{\mathrm{R}}}\right) = \frac{\varrho}{2}\left(b_{\mathrm{MISE},K_{\mathrm{L}}} + b_{\mathrm{MISE},K_{\mathrm{R}}}\right) + o_P\left(n^{-1/5}\right) = b_{\mathrm{MISE},K} + o_P\left(n^{-1/5}\right)$. *With respect to BO-validation, note that we can write the indirect estimator,* $\widehat{\alpha}_{b,K}^{\mathrm{BO}}$*, as a linear combination of two local linear estimators, one with left-sided kernel,* $K_{\mathrm{L}}$*, and the other with right-sided kernel,* $K_{\mathrm{R}}$*, that is*

$$\widehat{\alpha}_{b,K}^{\mathrm{BO}}(t) = \widehat{\alpha}_{b,K_{\mathrm{L}}}(t)\xi_b(t) + \widehat{\alpha}_{b,K_{\mathrm{R}}}(t)\left(1 - \xi_b(t)\right),$$

*and we have that* $\xi_b(t)$ *tends to zero as* $n \to +\infty$*, so asymptotically we have that the indirect local linear estimator for BO-validation is just the local linear estimator with right-sided kernel, which in turns, asymptotically equals the left-sided version. Thus the conclusion of Lemma 5 is also valid for BO-validation.*

**First and second derivative of the ISE**

**Lemma 6** *Under Assumptions A1–A3 we obtain the following, uniformly in* $b \in I_n$,

$$\begin{aligned} D'_L(b) &= n^{-2}b^{-2}\int\int G_L\left(b^{-1}(u-v)\right)\gamma^{-1}(u)w(u)dM(u)dM(v) + \\ &+ 2n^{-1}b\mu_2\left(\bar{L}^*\right)\int \alpha''(u)w(u)dM(u) + o_P\left(n^{-7/10}\right); \end{aligned} \tag{11}$$

$$\begin{aligned} \Delta'_L(b) &= n^{-2}b^{-2}\int\int H_L\left(b^{-1}(u-v)\right)\gamma^{-1}(u)w(u)dM(u)dM(v) + \\ &+ 2n^{-1}b\mu_2\left(\bar{L}^*\right)\int \alpha''(u)w(u)dM(u) + o_P\left(n^{-7/10}\right); \end{aligned} \tag{12}$$

*where* $H_L(u) = I[u \neq 0]\int \bar{L}^*(v)\left[\bar{L}_1^*(u+v) + \bar{L}_1^*(-u+v)\right]dv$*, and* $G_L(u) = 2I[u \neq 0]\bar{L}_1^*(u)$*, with* $\bar{L}_1^*(u) = -\bar{L}^*(u) - u\bar{L}^{*\prime}(u)$*, and*

$$\begin{aligned} \Delta''_L(b) &= 3b^2\mu_2\left(\bar{L}^*\right)^2\int \alpha''(t)^2\gamma(t)w(t)dt + \\ &\qquad 2n^{-1}b^{-3}R\left(\bar{L}^*\right)\int \alpha(t)w(t)dt + o_P\left(n^{-4/10}\right). \end{aligned} \tag{13}$$

*Proof.* The error of the leave-one-out estimator can be decomposed as the sum of the corresponding variance and bias terms, as usual, and then differentiate with respect to $b$. Hence,

$$\begin{aligned} D'_L(b) &= 2n^{-1}\int\int \partial_b\bar{L}_{t,b}(t-s)I(s \neq t)w(t)dM(t)dM(s) + 2n^{-1}\int \partial_b B_{b,L}(t)w(t)dM(t) \\ &= D'_{1,L}(b) + D'_{2,L}(b) \end{aligned}$$

where we mean $\partial_b = \frac{\partial}{\partial b}$.

Following arguments in Lemma 4 of Gamiz et al. (2016) we can replace $\bar{L}_{t,b}$ and $\partial_b\bar{L}_{t,b}$

by the kernel $Y^{-1}(t)\bar{L}_b^*$ and $Y^{-1}(t)\partial_b\bar{L}_b^*$, respectively, so we can write

$$\begin{aligned} D'_{1,L}(b) &= -2n^{-2}b^{-2}\int\int\left\{\bar{L}^*\left(\frac{t-s}{b}\right)+\left(\frac{t-s}{b}\right)\bar{L}^{*'}\left(\frac{t-s}{b}\right)\right\} \\ &\quad \times I(s\neq t)\gamma(t)^{-1}w(t)dM(t)dM(s)+o_P\left(n^{-7/10}\right) \\ &= n^{-2}b^{-2}\int\int G_L\left(\frac{t-s}{b}\right)\gamma(t)^{-1}w(t)dM(t)dM(s)+o_P\left(n^{-7/10}\right), \end{aligned}$$

with $G_L$ defined above.

As for the second term $D'_{2,L}=2n^{-1}b\mu_2\left(\bar{L}^*\right)\int\alpha''(t)w(t)dM(t)$.

To obtain the first derivative of the ISE we consider

$$\begin{aligned} \Delta'_L(b) &= 2n^{-1}\int V_{b,L}(t)\partial_b V_{b,L}(t)w(t)Y(t)dt+ \\ &+ 2n^{-1}\int\left(V_{b,L}(t)\partial_b B_{b,L}(t)+B_{b,L}(t)\partial_b V_{b,L}(t)\right)w(t)Y(t)dt \\ &+ 2n^{-1}\int B_{b,L}(t)\partial_b B_{b,L}(t)w(t)Y(t)dt \end{aligned}$$

The last term is of lower order, i.e., $n^{-2}b^3$, so we do not consider it in what follows. Regarding the first term we have

$$\Delta'_{1,L}(b)=2\int\int\int\bar{L}_{t,b}(t-s)\partial_b\bar{L}_{t,b}(t-u)w(t)\gamma(t)dtdM(s)dM(u)$$

Again we can replace $\bar{L}_{t,b}$ and $\partial_b\bar{L}_{t,b}$ by the kernel $Y^{-1}(t)\bar{L}_b^*$ and $Y^{-1}(t)\partial_b\bar{L}_b^*$, respectively, and then

$$\begin{aligned} \Delta'_{1,L}(b) &= 2n^{-2}\int\int\int\bar{L}_b^*(t-s)\partial_b\bar{L}_b^*(t-u)w(t)\gamma(t)^{-1}dtdM(s)dM(u) \\ &+ o_P\left(n^{-7/10}\right), \end{aligned}$$

which can be written

$$\begin{aligned} \Delta'_{1,L}(b) &= \int\int\int\left\{\bar{L}_b^*(t-s)\partial_b\bar{L}_b^*(t-u)+\bar{L}_b^*(t-u)\partial_b L_b^*(t-s)\right\}I(s\neq u) \\ &\quad \times w(t)\gamma(t)^{-1}dtdM(s)dM(u)+o_P\left(n^{-7/10}\right). \end{aligned}$$

After a convenient change of variable in the integral we get

$$\begin{aligned}\Delta'_{1,L}(b) &= \int\int\left[\int \bar{L}^*(v)\left(\bar{L}_1^*\left(v+\frac{s-u}{b}\right)+\bar{L}_1^*\left(v-\frac{s-u}{b}\right)\right)I(s\neq u)dv\right]\\ &\quad\times w(u)\gamma(u)^{-1}dtdM(s)dM(u)+o_P\left(n^{-7/10}\right),\end{aligned}$$

then define $H_L(u) = I[u\neq 0]\int \bar{L}^*(v)\left[\bar{L}_1^*(u+v)+\bar{L}_1^*(-u+v)\right]dv$ to obtain the first term in (12). For the second term in $\Delta'_L$ we derive with respect to $b$ and change the order of the integrals.

Finally, we obtain the expression of the second derivative of the ISE given in (13) using similar arguments as in Lemma 4, and replacing $\bar{L}_{t,b}$ and its derivatives by $\bar{L}^+_{t,b}$ and its derivatives, which leads to terms of order $o_P\left(n^{-2/5}\right)$. Then we replace the kernel $\bar{L}^+_{t,b}(t-s)$ by $Y^{-1}(t)\bar{L}^*_b(t-s)$ and obtain the corresponding derivatives. □

**Remark 2** *As consequence of Lemma 6 we can write for* $b = b_{\text{MISE},L}$*,* $M''_L(b) = n^{\frac{-2}{5}}C_{1,L}$*, where*

$$\begin{aligned}C_{1,L} &= 5\left(R\left(\bar{L}^*\right)\right)^{2/5}\left(\mu_2\left(\bar{L}^*\right)\right)^{6/5}\\ &\quad\times\left(\int\alpha(u)w(u)du\right)^{2/5}\left(\int\alpha''(u)^2\gamma(u)w(u)du\right)^{3/5}.\end{aligned}$$

**Proof of Theorem 1**

Using a Taylor expansion we get

$$\begin{aligned}\widehat{b}_{\text{CV},L}-b_{\text{MISE},L} &= -\left(M''_L(b^*)\right)^{-1}\widehat{\Delta}'_L\left(b_{\text{MISE},L}\right)+o_P\left(n^{-3/10}\right),\\ \widehat{b}_{\text{ISE},L}-b_{\text{MISE},L} &= -\left(M''_L(b^{**})\right)^{-1}\Delta'_L\left(b_{\text{MISE},L}\right)+o_P\left(n^{-3/10}\right),\end{aligned}$$

for $b^*$ a bandwidth between $\widehat{b}_{\mathrm{CV},L}$ and $b_{\mathrm{MISE},L}$, whereas $b^{**}$ is a bandwidth between $\widehat{b}_{\mathrm{ISE},L}$ and $b_{\mathrm{MISE},L}$. Now we use continuity of $M''_{\mathrm{L}}$ and that $M''_{\mathrm{L}}(b_{\mathrm{MISE},L}) = C_{1,L}n^{-2/5}$, then we have

$$\begin{aligned}\widehat{b}_{\mathrm{CV},L} - b_{\mathrm{MISE},L} &= -n^{-8/5}C_{1,L}^{-1}b^{-2} \\ &\int\int (H_L - G_L)\left(\frac{u-v}{b}\right)\gamma^{-1}(u)w(u)dM(u)dM(v) + o_P\left(n^{-3/10}\right),\end{aligned} \tag{14}$$

and,

$$\begin{aligned}\widehat{b}_{\mathrm{ISE},L} - b_{\mathrm{MISE},L} &= -n^{-8/5}C_{1,L}^{-1}b^{-2}\int\int H_L\left(\frac{u-v}{b}\right)\gamma^{-1}(u)w(u)dM(u)dM(v) \\ &+ 2n^{-3/5}C_{1,L}^{-1}\, b\mu_2\left(\bar{L}^*\right)\int \alpha''(u)w(u)dM(u) + o_P\left(n^{-3/10}\right),\end{aligned} \tag{15}$$

where for short in the expressions above we put $b = b_{\mathrm{MISE},L}$. For the case of cross-validation, putting $b = b_{\mathrm{MISE},K}$ we have

$$\begin{aligned}\widehat{b}_{\mathrm{CV},K} - \widehat{b}_{\mathrm{ISE},K} &= C_{1,K}^{-1}n^{-8/5}b^{-2}\int\int G_K\left(\frac{u-v}{b}\right)\gamma^{-1}(u)w(u)dM(u)dM(v) + \\ &2n^{-3/5}C_{1,K}^{-1}\, b\mu_2\left(\bar{L}^*\right)\int \alpha''(u)w(u)dM(u) + o_P\left(n^{-3/10}\right).\end{aligned}$$

For DO-validation we have that $\widehat{b}_{\mathrm{DO,K}} = \rho(\widehat{b}_{\mathrm{CV},K_{\mathrm{L}}} + \widehat{b}_{\mathrm{CV},K_{\mathrm{R}}})/2$, then we can write

$$\widehat{b}_{\mathrm{DO},K} - \widehat{b}_{\mathrm{ISE},K} = \frac{\rho}{2}\left(\widehat{b}_{\mathrm{CV},K_{\mathrm{L}}} - b_{\mathrm{MISE},K_{\mathrm{L}}}\right) + \frac{\rho}{2}\left(\widehat{b}_{\mathrm{CV},K_{\mathrm{R}}} - b_{\mathrm{MISE},K_{\mathrm{R}}}\right) + \left(b_{\mathrm{MISE},K} - \widehat{b}_{\mathrm{ISE},K}\right).$$

Using that $b_{\mathrm{MISE},K} = \rho b_{\mathrm{MISE},L}$, for $L = K_{\mathrm{L}}, K_{\mathrm{R}}$, and given that $C_{1,K_{\mathrm{L}}} = C_{1,K_{\mathrm{R}}}$, from expression (14) we can write

$$\begin{aligned}\widehat{b}_{\mathrm{DO},K} - \widehat{b}_{\mathrm{ISE},K} &= -n^{-8/5}b^{-2}\int\int\left\{C_{1,K_{\mathrm{L}}}^{-1}\frac{\rho^3}{2}\left((H_{K_{\mathrm{L}}} - G_{K_{\mathrm{L}}}) + (H_{K_{\mathrm{R}}} - G_{K_{\mathrm{R}}})\right)\left(\frac{u-v}{b\rho^{-1}}\right)\right. \\ &\left. - C_{1,K}^{-1}H_K\left(\frac{u-v}{b}\right)\right\}\gamma^{-1}(u)w(u)dM(u)dM(v) \\ &-2n^{-3/5}C_{1,K}^{-1}b\mu_2(K)\int \alpha''(u)w(u)dM(u) + o_P\left(n^{-3/10}\right).\end{aligned} \tag{16}$$

It can be checked that $\rho^3 C_{1,L}^{-1} = \frac{R(\bar{K}^*)}{R(\bar{L}^*)} C_{1,K}^{-1}$, so we can rewrite the integrand of the first term in expression (16) accordingly, and we obtain the DO-validation case also having into account that $R\left(\bar{K}_{\mathrm{L}}\right) = R\left(\bar{K}_{\mathrm{R}}\right)$ and $\mu_2\left(\bar{K}_{\mathrm{L}}\right) = \mu_2\left(\bar{K}_{\mathrm{R}}\right)$.

Finally, as explained in Remark 1, the indirect estimator for BO-validation behaves as the left-one side (equivalently right-one side) version of the estimator for $n \to +\infty$, then we can take $\widehat{b}_{\mathrm{BO},K} = \rho \widehat{b}_{\mathrm{CV},K_{\mathrm{L}}}$, for example, and then use (14).

This concludes the proof of Theorem 1. □

## 1.4 Asymptotics of bandwidth selectors for a multiplicative bias corrected estimator

Consider now the multiplicative bias corrected (MBC) estimator, $\widehat{\alpha}_{b,L}^{\mathrm{MBC}}$, with bandwidth $b$ and kernel $L$, given by

$$\widehat{\alpha}_{b,L}^{\mathrm{MBC}}(t) = \sum_{i=1}^{n} \int \bar{L}_{t,b}^{\mathrm{MBC}}(t-s) \widehat{\alpha}_{b,L}^{\mathrm{LL}}(t) (\widehat{\alpha}_{b,L}^{\mathrm{LL}}(s))^{-1} dN_i(s), \tag{17}$$

with stochastic kernel

$$\bar{L}_{t,b}^{\mathrm{MBC}}(t-s) = \frac{a_{2,L}^{\mathrm{MBC}}(t) - a_{1,L}^{\mathrm{MBC}}(t)(t-s)}{a_{0,L}^{\mathrm{MBC}}(t) a_{2,L}^{\mathrm{MBC}}(t) - (a_{1,L}^{\mathrm{MBC}}(t))^2} \left(\widehat{\alpha}_{b,L}^{\mathrm{LL}}(s)\right)^2 L_b\left(t-s\right), \tag{18}$$

where $a_{j,L}^{\mathrm{MBC}}(t) = \int_0^T L_b\left(t-s\right)\left(t-s\right)^j \left(\widehat{\alpha}_{b,L}^{\mathrm{LL}}(s)\right)^2 Y(s) ds$, for $j = 0, 1, 2$.

Recall the decomposition

$$\widehat{\alpha}_{b,L}^{\mathrm{MBC}}(t) - \alpha(t) = B_{b,L}^{\mathrm{MBC}}(t) + V_{b,L}^{\mathrm{MBC}}(t),$$

where we have defined

$$B_{b,L}^{\mathrm{MBC}}(t) = \int \bar{L}_{t,b}^{\mathrm{MBC}}(t-s) \widehat{\alpha}_{b,L}^{\mathrm{LL}}(t) \left(\beta_{b,L}(t) - \beta_{b,L}(s)\right) Y(s) ds, \tag{19}$$

with $\beta_{b,L}(s) = (\widehat{\alpha}^{\mathrm{LL}}_{b,L}(s))^{-1} B^{\mathrm{LL}}_{b,L}(s)$, and $B^{\mathrm{LL}}_{b,L}$ given in (4); and

$$V^{\mathrm{MBC}}_{b,L}(t) = \int f^{\mathrm{MBC}}_{t,b}(s) dM(s), \tag{20}$$

where

$$\begin{aligned} f^{\mathrm{MBC}}_{t,b}(s) &= \bar{L}^{\mathrm{MBC}}_{t,b}(t-s)\frac{\widehat{\alpha}^{\mathrm{LL}}_{b,L}(t)}{\widehat{\alpha}^{\mathrm{LL}}_{b,L}(s)} + \bar{L}_{t,b}(t-s) - \\ & \int_0^T \bar{L}^{\mathrm{MBC}}_{t,b}(t-u)\frac{\widehat{\alpha}^{\mathrm{LL}}_{b,L}(t)}{\widehat{\alpha}^{\mathrm{LL}}_{b,L}(u)}\bar{L}_{u,b}(u-s)Y(u)du. \end{aligned} \tag{21}$$

Similarly to the local linear case, to prove Theorem 2 we first state a uniform expansion for the ISE. For the estimator $\widehat{\alpha}^{\mathrm{MBC}}_{b,L}$ the ISE is defined as

$$\Delta^{\mathrm{MBC}}_{L}(b) = n^{-1}\int_0^T \left(\widehat{\alpha}^{\mathrm{MBC}}_{b,L}(t) - \alpha(t)\right)^2 w(t)Y(t)dt.$$

We assume that the minimizer of the ISE above, $\widehat{b}^{\mathrm{MBC}}_{\mathrm{ISE},L}$, is calculated over the interval $I^{\mathrm{MBC}}_n = \left[c_1 n^{-1/9}, c_2 n^{-1/9}\right]$, where constants $0 < c_1 < c_2$ are chosen such that $c_1 < C^{\mathrm{MBC}}_{0,L} < c_2$, where

$$C^{\mathrm{MBC}}_{0,L} = \left[\frac{R\left(\Gamma_{\bar{L}^*}\right)\int \alpha(t)w(t)dt}{\frac{\left(\mu_2(\bar{L}^*)\right)^4}{2}\int (h(t))^2\gamma(t)w(t)dt}\right]^{1/9},$$

with $\Gamma_{\bar{L}^*}(u) = 2\bar{L}^*(u) - \bar{L}^*(u) * \bar{L}^*(u)$; and, $h(t) = \alpha(t)\left(\alpha''(t)/\alpha(t)\right)''$.

For simplicity we remove hereafter in this section the superscript MBC and write $\widehat{\alpha}^{\mathrm{MBC}}_{b,L} = \widehat{\alpha}_{b,L}$, $\Delta^{\mathrm{MBC}}_{L} = \Delta_L$, $B^{\mathrm{MBC}}_{b,L} = B_{b,L}$, $V^{\mathrm{MBC}}_{b,L} = V_{b,L}$, $f^{\mathrm{MBC}}_{t,b} = f_{t,b}$, $I^{\mathrm{MBC}}_n = I_n$ and $C^{\mathrm{MBC}}_{0,L} = C_{0,L}$.

**Asymptotic expansion of the ISE**

**Lemma 7** *Under Assumptions A1, A2' and A3', we have the following expansion of the ISE of the MBC estimator with kernel L and bandwidth b,*

$$\Delta_L(b) = M_L(b) + o_P((nb)^{-1}) = M_L(b) + o_P(n^{-8/9}),$$

*uniformly for* $b \in I_n$, *where*

$$M_L(b) = b^8 \frac{\mu_2^4\left(\bar{L}^*\right)}{16} \int (h(t))^2 \gamma(t) w(t) dt + (nb)^{-1} R\left(\Gamma_{\bar{L}^*}\right) \int \alpha(t) w(t) dt$$

*with* $h(t) = \alpha(t)\left(\alpha''(t)/\alpha(t)\right)''$.

*Proof.*

$$\begin{aligned}
\Delta_L(b) &= n^{-1} \int_0^T \left(V_{b,L}(t) + B_{b,L}(t)\right)^2 w(t) Y(t) dt = \\
&= n^{-1} \int_0^T \left(V_{b,L}(t)\right)^2 w(t) Y(t) dt + 2n^{-1} \int_0^T V_{b,L}(t) B_{b,L}(t) w(t) Y(t) dt + \\
&+ n^{-1} \int_0^T \left(B_{b,L}(t)\right)^2 w(t) Y(t) dt.
\end{aligned}$$

with $B_{b,L}(t)$ and $V_{b,L}(t)$ given in (19) and (20), respectively.

We treat the terms in $\Delta_L(b)$ separately, and using Assumption A2', we can write

$$\Delta_L(b) = S_{L,1}(b) + S_{L,2}(b) + T_{L,1}(b) + T_{L,2}(b) + o_P(1),$$

where we define

$$\begin{aligned}
S_{L,1}(b) &= \int_0^T \int_0^T \bar{H}_{L,b}(u,v) dM(u) dM(v) - \int_0^T \bar{H}_{L,b}(u,u) \alpha(u) Y(u) du \\
S_{L,2}(b) &= \int_0^T \delta_{L,b}(u) dM(u) \\
T_{L,1}(b) &= \int_0^T \bar{H}_{L,b}(u,u) \alpha(u) Y(u) du \\
T_{L,2}(b) &= \int_0^T \left(B_{b,L}(t)\right)^2 w(t) \gamma(t) dt
\end{aligned}$$

with $\bar{H}_{L,b}(u,v) = \int_0^T f_{t,b}(u)\ f_{t,b}(v)\ w(t)\gamma(t)dt$, and $\delta_{b,L}(u) = 2\int_0^T f_{t,b}(u)\ B_{b,L}(t) w(t) \gamma(t) dt$.

Now we define the following processes

$$\begin{aligned} S_{L,1,t}(z) &= n^{8/9}\int_0^t\int_0^t \bar{H}_{L,zn^{-1/9}}(u,v)dM(u)dM(v) - n^{8/9}\int_0^t \bar{H}_{L,zn^{-1/9}}(u,u)\alpha(u)Y(u)du = \\ &= n^{8/9}\int_0^t\int_0^v \left(\bar{H}_{L,zn^{-1/9}}(u,v)+\bar{H}_{L,zn^{-1/9}}(v,u)\right) I(u\neq v)dM(u)dM(v) = \\ &= n^{8/9}\int_0^t\int_0^v 2\bar{H}_{L,zn^{-1/9}}(u,v)I(u\neq v)dM(u)dM(v), \end{aligned}$$

and

$$S_{L,2,t}(z) = n^{8/9}\int_0^t \delta_{L,zn^{-1/9}}(u)dM(u),$$

for $z\in[c_1,c_2]$.

The function $f_{t,b}$ which is involved in the integrands of $S_{L,1,t}$ and $S_{L,2,t}$ is not predictable so we cannot directly apply Theorem 3 to these processes. However we can follow similar arguments as in Mammen and Nielsen (2007) to show that the asymptotic properties of $S_{L,1,t}$ and $S_{L,2,t}$ are the same as for the following processes

$$S^*_{L,1,t}(z) = n^{8/9}\int_0^t\int_0^v 2\bar{H}^*_{L,zn^{-1/9}}(u,v)I(u\neq v)dM(u)dM(v), \tag{22}$$

and

$$S^*_{L,2,t}(z) = n^{8/9}\int_0^t \delta^*_{L,zn^{-1/9}}(u)dM(u),$$

with $\bar{H}^*_{L,b}(u,v) = \int_0^T f^*_{t,b}(u)\ f^*_{t,b}(v)\ w(t)\gamma(t)dt$, and $\delta^*_{L,b}(u) = 2\int_0^T f^*_{t,b}(u)B_{b,L}(t)w(t)\gamma(t)dt$, where we have replaced $f_{t,b}$ given in (21) by $f^*_{t,b}$ defined as

$$f^*_{t,b}(s) = \left\{2\bar{L}^*_b(t-s) - \int \bar{L}^*_b(t-u)\bar{L}^*_b(u-s)du\right\}\gamma(t)^{-1}n^{-1}, \tag{23}$$

with $\bar{L}^*_b(u) = b^{-1}\bar{L}^*(u/b)$, and $\bar{L}^*$ given in (5). Specifically we can use Lemma A1 of Mammen and Nielsen (2007) to obtain that

$$(nb)\left\{\int_0^v \left(\bar{H}^*_{L,b}(u,v) - \bar{H}_{L,b}(u,v)\right)dM(u)\right\} = o_P(1),$$

and

$$(nb)\left\{\int_0^t \left(\delta^*_{L,b}(u)-\delta_{L,b}(u)\right)dM(u)\right\} = o_P(1),$$

Then, we can apply Theorem 3 for $\sigma^2 = 0$ and get pointwise convergence to zero, $S^*_{L,1,T}(z) = o_P(1)$ and $S^*_{L,2,T}(z) = o_P(1)$. The uniform convergence to zero follows from the tightness of functions $S^*_{L,1,T}(z)$ and $S^*_{L,2,T}(z)$. Then we conclude that

$$S_{L,1}(b) = o_P\left(n^{-8/9}\right), \text{ and } S_{L,2}(b) = o_P\left(n^{-8/9}\right), \text{ uniformly in } b \in I_n.$$

To finish the proof it is not difficult to obtain that

$$T_{L,1}(b) = (nb)^{-1}R\left(\Gamma_{\bar{L}^*}\right)\int \alpha(t)w(t)dt + o_P\left((nb)^{-1}\right),$$

and

$$T_{L,2}(b) = b^8\frac{\left(\mu_2\bar{L}^*\right)^4}{16}\int \left(h(t)\right)^2\gamma(t)w(t)dt + o_P\left(b^8\right).$$

□

**Consistency of cross-validation**

The following lemma states consistency of the cross-validated bandwidth $\widehat{b}_{\mathrm{CV},L}$ for a general kernel $L$, and as a consequence the consistency of the BO-validated bandwidth for the MBC estimator.

**Lemma 8** *Under assumptions A1, A2' and A3', we have that* $\widehat{b}_{\mathrm{CV},L} = b_{\mathrm{MISE,L}} + o_P\left(n^{-1/9}\right)$.

*Proof.*

First we write the ISE in terms of the cross-validation score, $\widehat{Q}_L(b)$, given in (9):

$$\begin{aligned}\Delta_L(b) = \widehat{Q}_L(b) \;&+\; n^{-1}\int \alpha^2(s)Y(s)w(s)ds - 2n^{-1}\int \widehat{\alpha}_{b,L}(s)\alpha(s)Y(s)w(s)ds + \\ &+\; 2n^{-1}\int \widehat{\alpha}^{-}_{b,L}(s)w(s)dN(s).\end{aligned}$$

with $\widehat{\alpha}_{b,L}^{-}(s)=\int_0^T \bar{L}_{t,b}(t-s)I(s\neq t)dN(t)$ and $\bar{L}_{t,b}$ being the MBC kernel in (18). We can decompose the last term on the right hand side of the previous expression, and thus write

$$\Delta_L(b)=\widehat{\Delta}_L(b)+D_L(b)$$

where

$$\widehat{\Delta}_L(b)=\widehat{Q}_L(b)+n^{-1}\int \alpha^2(s)Y(s)w(s)ds+2n^{-1}\int \alpha(s)dM(s).$$

and

$$\begin{aligned} D_L(b) &= 2n^{-1}\int \left(\widehat{\alpha}_{b,L}^{-}(s)-\widehat{\alpha}_{b,L}(s)\right)\alpha(s)Y(s)w(s)ds+2n^{-1}\int \left(\widehat{\alpha}_{b,L}^{-}(s)-\alpha(s)\right)w(s)dM(s) \\ &= 2n^{-1}\int \left(\widehat{\alpha}_{b,L}^{-}(s)-\alpha(s)\right)w(s)dM(s). \end{aligned} \tag{24}$$

Note that $\widehat{\Delta}_L(b)$ has the same minimizer than $\widehat{Q}_L(b)$, then it is sufficient to show that $D_L(b)=o_P\left(n^{-8/9}\right)$, uniformly for $b\in I_n$. which can be obtained by similar arguments as Lemma 2 of Gámiz et al. (2016). Then we deduce that $\widehat{b}_{\mathrm{CV},L}=b_{\mathrm{MISE},L}+o_P\left(n^{-1/9}\right)$.

□

**First and second derivative of the ISE**

**Lemma 9** *Under A1, A2' and A3', we get that, uniformly in $b\in I_n$,*

$$\begin{aligned} \Delta'(b) &= n^{-2}b^{-2}\int H_L(b^{-1}(u-v))w(u)\gamma(u)^{-1}\ dM(u)\ dM(v) \\ &\qquad +n^{-1}b^3\mu_2^2\left(\Gamma_{\bar{L}^*}\right)\int \left(\frac{\alpha''(u)}{\alpha(u)}\right)''\alpha(u)w(u)\ dM(u)+o_P\left(n^{-15/18}\right), \end{aligned}$$

*where*

$$H_L(v)=I(v\neq 0)\int \Gamma_{\bar{L}^*}(u)\left\{\Gamma_{1,\bar{L}^*}(v+u)+\Gamma_{1,\bar{L}^*}(-v+u)\right\}du,$$

*with* $\Gamma_{1,\bar{L}^*}(u) = -\Gamma_{\bar{L}^*}(u) - u\Gamma'_{\bar{L}^*}(u)$*; and,*

$$\begin{aligned} D_1'(b) &= n^{-2}b^{-2}\int G_L(b^{-1}(u-v))\gamma(u)^{-1}\, dM(u)\, dM(v) \\ &\quad + n^{-1}b^3\left(\mu_2\left(\Gamma_{\bar{L}^*}\right)\right)^2 \int \left(\frac{\alpha''(u)}{\alpha(u)}\right)'' \alpha(u)w(u)\, dM(u) + o_P\left(n^{-15/18}\right), \end{aligned}$$

*where* $G_L(v) = 2I(v \neq 0)\Gamma_{1,\bar{L}^*}(v)$*, and*

$$\Delta_L''(b) = \frac{7}{2}b^6\mu_2^4\left(\bar{L}^*\right)\int\left(\left(\frac{\alpha''(t)}{\alpha(t)}\right)''\alpha(t)\right)^2\gamma(t)w(t)dt + 2n^{-1}b^{-3}R\left(\Gamma_{\bar{L}^*}\right)\int\alpha(t)w(t)dt + o_P\left(n^{-6/9}\right).$$

*Proof.* As in the local linear case, we decompose the error of the leave-one-out MBC estimator as the sum of the corresponding variance and bias terms, and then differentiate with respect to $b$. Hence,

$$\begin{aligned} D_L'(b) &= 2n^{-1}\int\int \partial_b f_{t,b}(s)I(s\neq t)w(t)dM(t)dM(s) + 2n^{-1}\int \partial_b B_{b,L}(t)w(t)dM(t) \\ &= D_{1,L}'(b) + D_{2,L}'(b). \end{aligned}$$

Following arguments in Lemma 4 of Gámiz et al. (2016) we can replace $f_{t,b}$ by $f_{t,b}^*$ so we get an error term of order $o_P\left(n^{-1}b^{-3/2}\right) = o_P\left(n^{-15/18}\right)$, and obtain

$$\begin{aligned} D_{1,L}'(b) &= 2n^{-2}b^{-2}\int\int\left\{\Gamma_{\bar{L}^*}\left(\frac{t-s}{b}\right) + \left(\frac{t-s}{b}\right)\Gamma'_{\bar{L}^*}\left(\frac{t-s}{b}\right)\right\} \\ &\quad \times I(s\neq t)\gamma(t)^{-1}w(t)dM(t)dM(s) + o_P\left(n^{-15/18}\right) \\ &= n^{-2}b^{-2}\int\int G_L\left(\frac{t-s}{b}\right)\gamma(t)^{-1}w(t)dM(t)dM(s) + o_P\left(n^{-15/18}\right). \end{aligned}$$

where we define $G_L(w) = 2\left(-\Gamma_{\bar{L}^*}(w) - w\Gamma'_{\bar{L}^*}(w)\right)I(w \neq 0)$. As for the second term $D_{2,L}' = 2n^{-1}b^3\left(\mu_2\left(\Gamma_{\bar{L}^*}\right)\right)^2\int h(t)w(t)dM(t) + o_P\left(n^{-15/18}\right)$, with $h(t) = \left(\alpha''(t)/\alpha(t)\right)''\alpha(t)$.

To obtain the first derivative of the ISE we consider

$$\begin{aligned}\Delta'_L(b) &= 2n^{-1}\int V_{b,L}(t)\partial_b V_{b,L}(t)w(t)Y(t)dt + \\ &+ 2n^{-1}\int \left(V_{b,L}(t)\partial_b B_{b,L}(t) + B_{b,L}(t)\partial_b V_{b,L}(t)\right) w(t)Y(t)dt \\ &+ 2n^{-1}\int B_{b,L}(t)\partial_b B_{b,L}(t)w(t)Y(t)dt\end{aligned}$$

The last term is of lower order, i.e. $n^{-2}b^3$, so we do not consider it in what follows. Regarding the first term we have

$$\Delta'_{1,L}(b) = 2\int\int\int f_{t,b}(s)\partial_b f_{t,b}(u)w(t)\gamma(t)dtdM(s)dM(u)$$

Again we can replace $f_{t,b}$ and $\partial_b f_{t,b}$ by $f^*_{t,b}$ and $\partial_b f^*_{t,b}$, respectively, and then

$$\begin{aligned}\Delta'_{1,L}(b) &= 2n^{-2}\int\int\int \Gamma_{\bar{L}^*,b}(t-s)\partial_b\Gamma_{\bar{L}^*,b}(t-u)w(t)\gamma(t)^{-1}dtdM(s)dM(u) \\ &+ o_P\left(n^{-15/18}\right),\end{aligned}$$

which can be written

$$\begin{aligned}\Delta'_{1,L}(b) &= \int\int\int \left\{\Gamma_{\bar{L}^*,b}(t-s)\partial_b\Gamma\bar{L}^*, b(t-u) + \Gamma_{\bar{L}^*,b}(t-u)\partial_b\Gamma_{L^*,b}(t-s)\right\} I(s\neq u) \\ &\quad \times w(t)\gamma(t)^{-1}dtdM(s)dM(u) + o_P\left(n^{-15/18}\right),\end{aligned}$$

with $\Gamma_{\bar{L}^*,b}(t-s) = 2\bar{L}^*_b(t-s) - \int \bar{L}^*_b(t-u)\bar{L}^*_b(u-s)du$.

After a convenient change of variable in the integral we get

$$\begin{aligned}\Delta_{1,L}(b) &= \int\int\left[\int \Gamma_{\bar{L}^*}(v)\left(\Gamma_{\bar{L}^*,1}\left(v+\frac{s-u}{b}\right) + \Gamma_{\bar{L}^*,1}\left(v-\frac{s-u}{b}\right)\right) I(s\neq u)dv\right] \\ &\quad \times w(u)\gamma(u)^{-1}dtdM(s)dM(u) + o_P\left(n^{-15/18}\right),\end{aligned}$$

with $\Gamma_{L,1}(u) = -\Gamma_L(u) - u\Gamma'_L(u)$. Then define

$$H_L(u) = I[u \neq 0] \int \Gamma_{\bar{L}^*}(v) \left[\Gamma_{\bar{L}^*,1}(u+v) + \Gamma_{\bar{L}^*,1}(-u+v)\right] dv$$

to obtain the first term in $\Delta'_L$. For the second term in $\Delta'_L$ we derive with respect to $b$ and change the order of the integrals.

Finally, we obtain the expression of the second derivative of the ISE using similar arguments as in Lemma 7, and replacing $f_{t,b}$ and its derivatives by $f^*_{t,b}$ and its derivatives, which leads to terms of order $o_P\left(b^6\right) = o_P\left(n^{-6/9}\right)$, for $b \in I_n$. □

**Remark 3** *As consequence of Lemma 9 we can write for* $b = b_{\text{MISE},L}$*,* $M''_L(b) = n^{\frac{-6}{9}} C_{1,L}$*, where*

$$\begin{aligned} C_{1,L} &= \frac{9}{2^{1/3}} \left(R\left(\Gamma_{\bar{L}^*}\right)\right)^{6/9} \left(\mu_2\left(\bar{L}^*\right)\right)^{12/9} \\ &\quad \times \left(\int \alpha(u)w(u)du\right)^{6/9} \left(\int h(u)^2\gamma(u)w(u)du\right)^{3/9}. \end{aligned}$$

□

## Proof of Theorem 2

Using a Taylor expansion we get

$$\begin{aligned} \widehat{b}_{\text{CV},L} - b_{\text{MISE},L} &= -\left(M''_L(b^*)\right)^{-1} \widehat{\Delta}'_L\left(b_{\text{MISE},L}\right) + o_P\left(n^{-3/18}\right), \\ \widehat{b}_{\text{ISE},L} - b_{\text{MISE},L} &= -\left(M''_L(b^{**})\right)^{-1} \Delta'_L\left(b_{\text{MISE},L}\right) + o_P\left(n^{-3/18}\right), \end{aligned}$$

for $b^*$ a bandwidth between $\widehat{b}_{\text{CV},L}$ and $b_{\text{MISE},L}$, whereas $b^{**}$ is a bandwidth between $\widehat{b}_{\text{ISE},L}$ and $b_{\text{MISE},L}$. Now we use continuity of $M''_{\text{L}}$ and that $M''_{\text{L}}(b_{\text{MISE},L}) = C_{1,L}n^{-6/9}$, then we have

$$\begin{aligned} \widehat{b}_{\text{CV},L} - b_{\text{MISE},L} &= -n^{-12/9} C_{1,L}^{-1} b^{-2} \\ &\quad \int\int \left(H_L - G_L\right)\left(\frac{u-v}{b}\right) \gamma^{-1}(u)w(u)dM(u)dM(v) + o_P\left(n^{-3/18}\right); \end{aligned} \tag{25}$$

and,

$$\begin{aligned}\widehat{b}_{\mathrm{ISE},L}-b_{\mathrm{MISE},L} &= -n^{-12/9}C_{1,L}^{-1}b^{-2}\int\int H_L\left(\frac{u-v}{b}\right)\gamma^{-1}(u)w(u)dM(u)dM(v)\\ &+ 2n^{-3/9}C_{1,L}^{-1}b^3\mu_2^2\left(\bar{L}^*\right)\int h(u)w(u)dM(u)+o_P\left(n^{-3/18}\right); \qquad (26)\end{aligned}$$

where for short in the expressions above we put $b = b_{\mathrm{MISE},L}$.

For the case of cross-validation, denoting $b = b_{\mathrm{MISE},K}$, we have

$$\begin{aligned}\widehat{b}_{\mathrm{CV},K}-\widehat{b}_{\mathrm{ISE},K} &= C_{1,K}^{-1}n^{-12/9}b^{-2}\int\int G_K\left(\frac{u-v}{b}\right)\gamma^{-1}(u)w(u)dM(u)dM(v)+\\ & 2n^{-3/9}C_{1,K}^{-1}b\mu_2^2\left(\bar{L}^*\right)\int h(u)w(u)dM(u)+o_P\left(n^{-3/18}\right).\end{aligned}$$

For DO-validation we have that $\widehat{b}_{\mathrm{DO,K}} = \rho(\widehat{b}_{\mathrm{CV,K_L}}+\widehat{b}_{\mathrm{CV,K_R}})/2$, then we can write

$$\widehat{b}_{\mathrm{DO},K}-\widehat{b}_{\mathrm{ISE},K}=\frac{\rho}{2}\left(\widehat{b}_{\mathrm{CV,K_L}}-b_{\mathrm{MISE,K_L}}\right)+\frac{\rho}{2}\left(\widehat{b}_{\mathrm{CV,K_R}}-b_{\mathrm{MISE,K_R}}\right)+\left(b_{\mathrm{MISE,K}}-\widehat{b}_{\mathrm{ISE,K}}\right).$$

Using that $b_{\mathrm{MISE},K} = \rho b_{\mathrm{MISE},L}$, for $L = K_{\mathrm{L}}, K_{\mathrm{R}}$, and given that $C_{1,K_{\mathrm{L}}} = C_{1,K_{\mathrm{R}}}$, from expression (25), we can write

$$\begin{aligned}\widehat{b}_{\mathrm{DO},K}-\widehat{b}_{\mathrm{ISE},K} &= -n^{-12/9}b^{-2}\int\int\Bigg\{C_{1,K_{\mathrm{L}}}^{-1}\frac{\rho^3}{2}\left(\left(H_{K_{\mathrm{L}}}-G_{K_{\mathrm{L}}}\right)+\left(H_{K_{\mathrm{R}}}-G_{K_{\mathrm{R}}}\right)\right)\left(\frac{u-v}{b\rho^{-1}}\right)\\ &\qquad - C_{1,K}^{-1}H_K\left(\frac{u-v}{b}\right)\Bigg\}\gamma^{-1}(u)w(u)dM(u)dM(v)\\ & -2n^{-3/9}C_{1,K}^{-1}b^3\mu_2^2(K)\int h(u)w(u)dM(u)+o_P\left(n^{-3/18}\right). \qquad (27)\end{aligned}$$

It can be checked that $\rho^3C_{1,L}^{-1} = \frac{R(\Gamma_{\bar{K}^*})}{R(\Gamma_{\bar{L}^*})}C_{1,K}^{-1}$, then we can re-write the integrand of the first term in expression (27) accordingly, so we obtain the DO-validation case also having into account that $R\left(\Gamma_{\bar{K}_{\mathrm{M}}}\right) = R\left(\Gamma_{\bar{K}_{\mathrm{R}}}\right)$ and $\mu_2\left(\bar{K}_{\mathrm{L}}\right) = \mu_2\left(\bar{K}_{\mathrm{R}}\right)$.

Finally, as explained in Remark 1, the indirect estimator for BO-validation behaves as the left-one side (equivalently right-one side) version of the estimator for $n\to+\infty$, then we can take $\widehat{b}_{\mathrm{BO},K} = \rho\widehat{b}_{\mathrm{CV},K_{\mathrm{L}}}$, for example, and then use (25).

This concludes the proof of Theorem 2. □

## 2 Additional plots for case studies and simulations

For the mortality case study, Figure 1 shows the scores for each bandwidth selection method considering the local linear estimator.

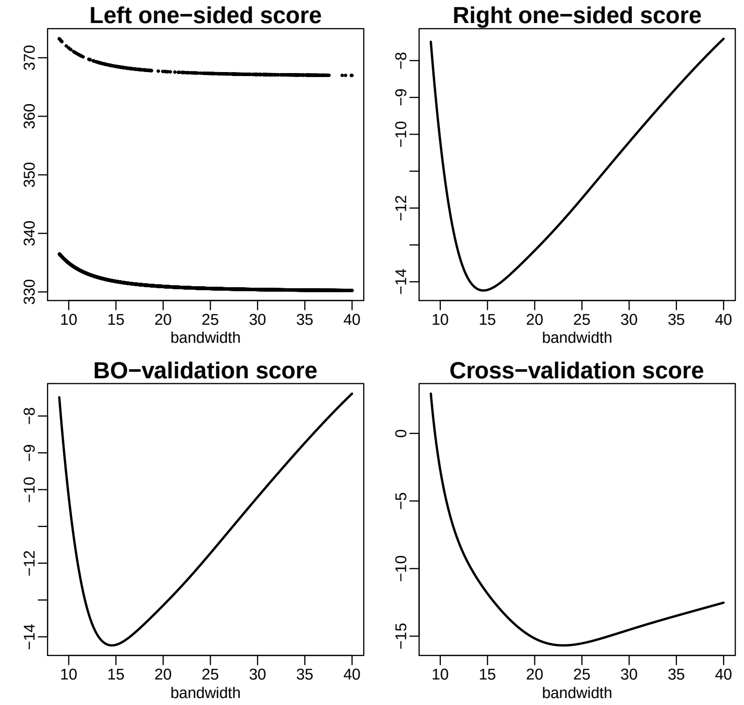


Figure 1: Mortality data: bandwidth selection scores with local linear hazard estimator.

For the application in non-life insurance, Figures 2 and 3 show the scores for the local linear hazard estimates of underwriting and reporting delay components, respectively.

In our simulations we have considered the five hazard models represented in Figure 4. The first four hazard functions are: $\alpha_1(t) = B(t, 2, 2)$, $\alpha_2(t) = B(t, 4, 4)$, $\alpha_3(t) = 0.6[B(t, 0.5, 0.5)+B(t, 7, 7)]$, $\alpha_4(t) = 0.6[B(t, 0.5, 0.5)+B(t, 4, 2)+B(t, 2, 4)]$. Here $B(t, a, b)$

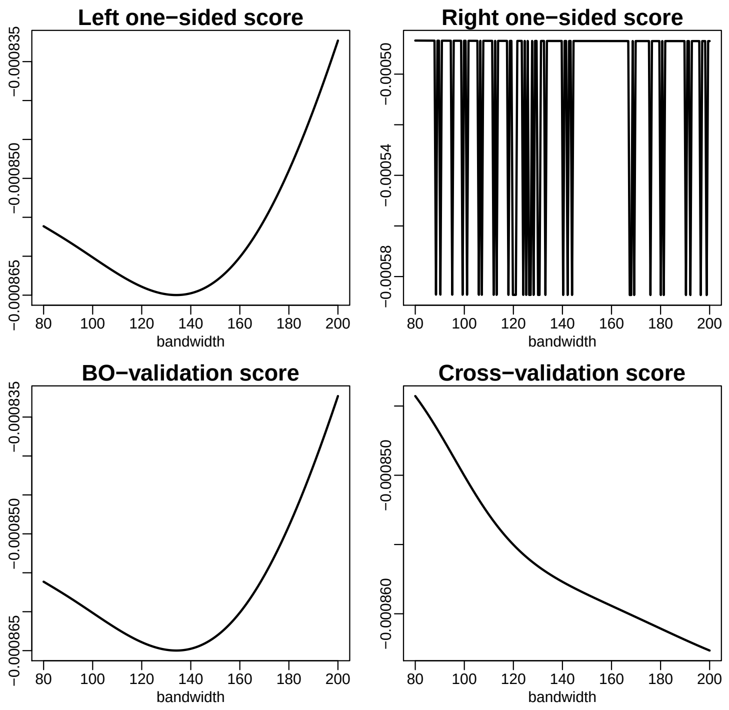


Figure 2: Underwriting component: bandwidth selection scores with LL estimator.

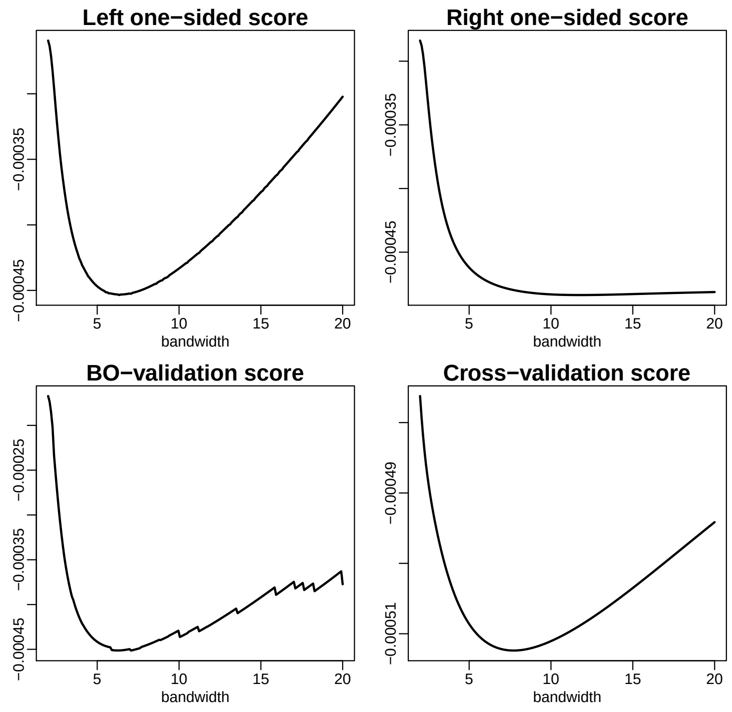


Figure 3: Reporting delay component: bandwidth selection scores with LL estimator.

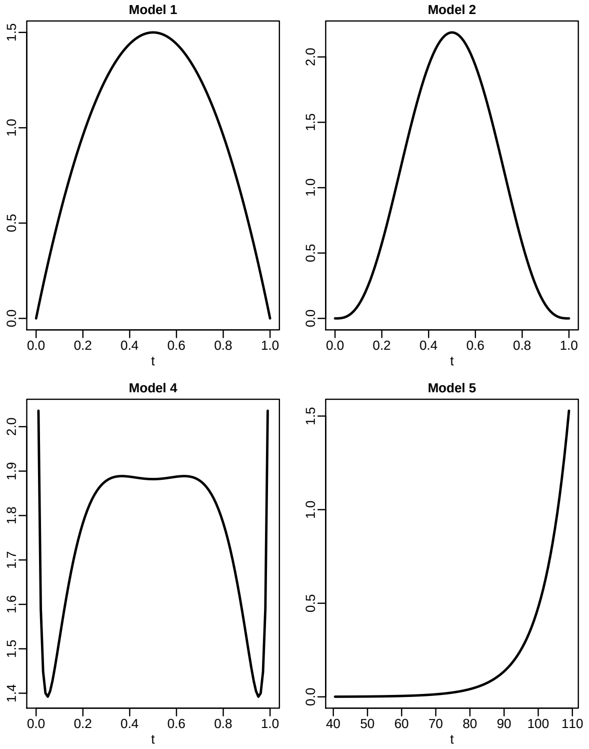


Figure 4: Simulated models: the true hazard functions.

is the density at $t$ of a Beta distribution with parameters $(a, b)$. The fifth hazard function is a mortality model which can be written as $\alpha_5(t) = (1+\sigma^2)^{-1} \exp(a_0+a_1t+a_2t^2)/\int_0^t \exp(a_0+a_1s + a_2s^2)ds$, where $a_0, a_1, a_2$ and $\sigma^2$ have been chosen as in the simulations of Gámiz et al. (2016).

Tables 1 and 2 summarize the simulations results for the five simulated models in the case of samples with right censoring and left truncation, and without left truncation, respectively. In these tables bandwidth estimates are compared according to the empirical MISE and two infeasible optimal bandwidths are considered as benchmarks: the ISE-optimal

bandwidth minimizing the ISE criterion and the MISE-optimal bandwidth minimizing the empirical MISE.

# References


Billingsley, P. (1968). *Convergence of probability measures.* New York: Wiley.

Gámiz, M. L., Mammen, E., Martínez-Miranda, M. D. and Nielsen, J. P. (2016). Double one-sided cross-validation of local linear hazards. *J. Royal Statist. Soc. B*, **78**, 755–779.

Hiabu, M., Mammen, E., Martínez-Miranda, M. D. and Nielsen, J. P. (2016) In-sample forecasting with local linear survival densities. *Biometrika*, **103**, 843–859.

Mammen, E. and Nielsen, J. P. (2007). A general approach to the predictability issue in survival analysis with applications. *Biometrika*, **94**, 873–892.

Ramlau-Hansen, H. (1983). Smoothing counting process intensities by means of kernel functions. *Ann. Statist.*, **11**, 453–466.

Table 1: Simulation results for datasets with right censoring and left truncation. The empirical MISE for each bandwidth estimate is shown (multiplied by $10^6$ for model 5 and by $10^4$ for the rest).

| | Local linear | | | | | MBC | | | | |
|---|---|---|---|---|---|---|---|---|---|---|
| | ISE | MISE | CV | DO | BO | ISE | MISE | CV | DO | BO |
| Model 1 | | | | | | | | | | |
| $n$ =100 | 9.7563 | 13.2635 | 18.3615 | 15.3183 | 16.6539 | 9.9505 | 11.9524 | 18.5897 | 15.8154 | 14.7824 |
| $n$ =1000 | 0.1321 | 0.1630 | 0.2342 | 0.1762 | 0.1831 | 0.1188 | 0.15 | 0.2459 | 0.2505 | 0.1629 |
| $n$ =10000 | 0.0023 | 0.0026 | 0.0030 | 0.0027 | 0.0027 | 0.0018 | 0.0022 | 0.0035 | 0.0028 | 0.0023 |
| Model 2 | | | | | | | | | | |
| $n$ =100 | 9.8719 | 12.336 | 18.4793 | 13.655 | 14.0958 | 10.3611 | 11.6265 | 19.6173 | 30.4656 | 14.1090 |
| $n$ =1000 | 0.1422 | 0.1608 | 0.2221 | 0.1752 | 0.1823 | 0.1265 | 0.1460 | 0.2419 | 0.9103 | 0.158 |
| $n$ =10000 | 0.0026 | 0.0028 | 0.0033 | 0.0029 | 0.0030 | 0.002 | 0.0022 | 0.0040 | 0.0080 | 0.0025 |
| Model 3 | | | | | | | | | | |
| $n$ =100 | 20.4410 | 27.5795 | 34.0625 | 27.7550 | 28.2916 | 19.1629 | 24.8769 | 31.5884 | 27.6015 | 28.9105 |
| $n$ =1000 | 0.4093 | 0.4887 | 0.7611 | 0.7743 | 0.7655 | 0.3314 | 0.4509 | 0.6097 | 0.6726 | 0.5643 |
| $n$ =10000 | 0.0097 | 0.0114 | 0.0167 | 0.0128 | 0.0130 | 0.0078 | 0.0098 | 0.0167 | 0.0120 | 0.0103 |
| Model 4 | | | | | | | | | | |
| $n$ =100 | 16.1049 | 18.792 | 38.1025 | 294.1373 | 35.6868 | 17.24 | 18.8492 | 22.725 | 19.8206 | 23.1987 |
| $n$ =1000 | 0.2364 | 0.2991 | 0.6964 | 0.4199 | 0.4773 | 0.2308 | 0.2785 | 0.4036 | 0.3060 | 0.3914 |
| $n$ =10000 | 0.0075 | 0.0095 | 0.0157 | 0.0113 | 0.012 | 0.0072 | 0.0089 | 0.0172 | 0.0098 | 0.0110 |
| Model 5 | | | | | | | | | | |
| $n$ =50000 | 0.1079 | 0.1287 | 0.1616 | 0.1410 | 0.1395 | 0.0585 | 0.0890 | 0.1468 | 0.1084 | 0.1008 |
| $n$ =75000 | 0.0488 | 0.0555 | 0.0715 | 0.0599 | 0.0592 | 0.0266 | 0.0386 | 0.0663 | 0.0547 | 0.0438 |
| $n = 10^5$ | 0.0313 | 0.0360 | 0.0432 | 0.0384 | 0.0382 | 0.0185 | 0.0251 | 0.0388 | 0.0374 | 0.0292 |

Table 2: Simulation results for datasets without left truncation. The empirical MISE for each bandwidth estimate is shown (multiplied by $10^6$ for model 5 and by $10^4$ for the rest).

| | Local linear | | | | | MBC | | | | |
|---|---|---|---|---|---|---|---|---|---|---|
| | ISE | MISE | CV | DO | BO | ISE | MISE | CV | DO | BO |
| Model 1 | | | | | | | | | | |
| $n$ =100 | 4.3365 | 5.0763 | 7.8430 | 5.6978 | 6.0487 | 4.4403 | 5.0850 | 9.2962 | 9.8927 | 6.3749 |
| $n$ =1000 | 0.0609 | 0.0710 | 0.0965 | 0.0745 | 0.0766 | 0.0561 | 0.0650 | 0.1150 | 0.1037 | 0.0689 |
| $n$ =10000 | 0.0010 | 0.0011 | 0.0014 | 0.0011 | 0.0011 | 8e-04 | 9e-04 | 0.0018 | 0.0014 | 9e-04 |
| Model 2 | | | | | | | | | | |
| $n$ =100 | 5.0990 | 6.1065 | 9.2904 | 6.7425 | 7.4117 | 5.7374 | 6.3250 | 11.2983 | 31.1161 | 7.6406 |
| $n$ =1000 | 0.0868 | 0.0970 | 0.1319 | 0.1035 | 0.1065 | 0.0676 | 0.0764 | 0.1354 | 0.7702 | 0.0869 |
| $n$ =10000 | 0.0015 | 0.0016 | 0.0019 | 0.0017 | 0.0017 | 9e-04 | 0.0011 | 0.0022 | 0.0059 | 0.0012 |
| Model 3 | | | | | | | | | | |
| $n$ =100 | 11.6357 | 12.5582 | 17.0835 | 15.2640 | 15.5297 | 11.4096 | 12.6480 | 18.1612 | 18.2355 | 21.0596 |
| $n$ =1000 | 0.2002 | 0.2111 | 0.2569 | 0.2211 | 0.2245 | 0.1703 | 0.1821 | 0.2457 | 0.2718 | 0.1925 |
| $n$ =10000 | 0.0039 | 0.0040 | 0.0045 | 0.0042 | 0.0042 | 0.0033 | 0.0034 | 0.0049 | 0.0058 | 0.0037 |
| Model 4 | | | | | | | | | | |
| $n$ =100 | 11.1611 | 12.8587 | 20.0296 | 15.5286 | 15.8548 | 11.2060 | 12.2018 | 14.0663 | 12.5113 | 13.7336 |
| $n$ =1000 | 0.1811 | 0.2142 | 0.3133 | 0.2443 | 0.2461 | 0.1716 | 0.1920 | 0.2419 | 0.2265 | 0.2497 |
| $n$ =10000 | 0.0053 | 0.0057 | 0.0068 | 0.0065 | 0.0065 | 0.0053 | 0.0059 | 0.0090 | 0.0089 | 0.0075 |
| Model 5 | | | | | | | | | | |
| $n$ =50000 | 1.1406 | 2.1607 | 13.3126 | 16.2856 | 3.0288 | 0.3318 | 0.7205 | 11.8369 | 2.4909 | 7.5344 |
| $n$ =75000 | 0.8244 | 1.3246 | 6.8173 | 10.2841 | 1.9197 | 0.2312 | 0.4317 | 5.7429 | 1.4218 | 3.0441 |
| $n = 10^5$ | 0.5262 | 0.8635 | 4.4354 | 7.5476 | 1.4309 | 0.1520 | 0.2729 | 3.5108 | 0.9591 | 1.6269 |
